# Supplementary material for: Enhancing Portuguese Variety Identification with Cross-Domain Approaches
Source: arXiv:2502.14394 source file (2025-02-20)
Supplement: Supplementary file 1 [file Appendix.tex]

\section{European and Brazilian Portuguese}
\label{app:pt_br_pt_pt}

The Portuguese language is an Indo-European, Romance and Iberian language with four branches of varieties: European, Brazilian, African and Asian that feature \textit{phonological}, \textit{morphological}, \textit{lexical}, \textit{syntactic}, and \textit{semantic} differences. Although the EP and BP varieties vary across all these linguistic levels, since our dataset considers exclusively written text, we will exclude the phonological differences from our analysis.

At the morpho-syntactic level, the contrast can be observed, for example, in the pronominal system and the structure of nominal, prepositional and verbal phrases. \citet{scherre2016main} discuss the variation in Brazilian Portuguese of the 2nd person singular (\textit{tu/ você}, ``you'') and 1st person plural (\textit{nós/ a gente}, ``we/the people'') nominative pronouns. Additionally,~\cite{kato2016european} show how the system and the position of clitics behave distinctively: while in EP, the clitics with the role of complement (\textit{o(s), a(s)} (``him'', her'', ``it'') are widely utilized (\textit{e.g. O João viu \underline{a Maria}/viu-a}, ``John saw Maria/her''), in BP, nominal phrase or the pronoun \textit{ele/ ela} (``he'', ``she'') are employed instead (e.g. \textit{O João viu \underline{Maria}/ ela}, ``John saw Maria/ she''). The position of the clitics is a factor of disparity between the two varieties as well because in EP the clitics are by default placed after the verb (enclisis), and in BP they are positioned before the verb (proclisis) (\textit{e.g. Dá-me um computador/ Me dá um computador}, ``Give me a computer'').

The contrast between the two varieties extends also to the structure of nominal and prepositional phrases. \citet{brit2016dp}, for instance, refers to the fact that in EP, the possessive is habitually preceded by a definite article, whereas in BP, it can occur by itself (e.g. \textit{O João viu \underline{a} minha filha/ minha filha}, ``John saw my daughter''). Moreover, BP allows for the use of a bare singular noun, which is disallowed in EP (e.g. \textit{Ontem vi filme no cinema} (EP$\times$; BP$\checkmark$), ``Yesterday, I saw a film at the cinema''). The expression of datives with the role of an indirect object is also built differently: whereas in EP, the preposition \textit{a} ('to') is used, in BP the preposition is another one, \textit{para} (``to''), as in \textit{O João contou \underline{à} Maria/para Maria} ('John told Maria'). Another well-known and documented morpho-syntactic difference lies in the opposition between using the infinitive versus gerund in constructions corresponding to the progressive or secondary predicates. In these cases, BP utilises the gerund while EP resorts to the infinitive (e.g. \textit{O João está \underline{a ler}/lendo}, ``John was reading''.

It is at the lexical level that the two varieties exhibit the most contrast. Besides the different words to represent the same entity (\textit{hospedeira de bordo/aeromoça}, ``stewardess''), Brazilian Portuguese has much vocabulary with indigenous (\textit{caipira, acajá}, and African (dengo, cafuné) origins. Brazilian lexical richness is also the result of the contact with the languages of numerous immigrants and the easiness in accepting neologisms and loanwords~\cite{silva2013portugues}.

The phonetic-phonological and prosodic differences are undoubtedly the most noticeable and some impact on orthography. When there is a stressed syllable followed by a nasal consonant at the beginning of the next syllable, the timbre of the stressed vowel varies depending on the variety: in EP  [\textopeno], [e] and in BP [o], [\textepsilon]. This phonetic feature is marked in writing with different orthographical signs, as illustrated in words like (\textit{homónimo/homônimo}, 'homonymous') and (\textit{grémio/grêmio}, 'guild'). Another case with consequences to the spelling refers to some consonants that are silent in one variety, but not in the other one, or the other way around, and that, when they are not silent, are represented orthographically (e.g. \textit{facto/fato}, 'fact' and \textit{ato/acto}, 'act'). Finally, in terms of orthography, certain specific words have different spellings in each variety, like (\textit{registo/registro}, 'registry').

\section{Implementation Details}
\label{app:hyper}

The NER and POS tags were identified using spaCy\footnote{\url{https://spacy.io/models/pt}}. The BERT model was trained with the \texttt{transformers}\footnote{\url{https://huggingface.co/docs/transformers/}} and \texttt{pytorch}\footnote{\url{https://pytorch.org}} libraries, using early stopping with a patience of three epochs, binary cross-entropy loss, and the AdamW optimizer. Additionally, a learning rate scheduler was used to reduce the learning rate by a factor of 0.1 if the training loss did not improve for two consecutive epochs. The N-grams models were trained using the \texttt{scikit-learn}\footnote{\url{https://scikit-learn.org/}} library. The hyperparameters searched for each model are detailed in Table~\ref{tab:hyperparameters}.

In Table~\ref{tab:hyperparameters} we list the additional parameters to delexicalization, considered during the grid search process.

\begin{table}
\centering
\begin{tblr}{
  colspec = {X[3,l]X[2,l]},
  width = \columnwidth,
  row{3} = {c},
  row{4} = {c},
  row{5} = {c},
  row{6} = {c},
  row{7} = {c},
  row{8} = {c},
  row{10} = {c},
  row{11} = {c},
  row{12} = {c},
  row{13} = {c},
  row{14} = {c},
  row{16} = {c},
  row{18} = {c},
  cell{1}{2} = {c},
  cell{2}{1} = {r=7}{},
  cell{2}{2} = {c},
  cell{9}{1} = {r=6}{},
  cell{9}{2} = {c},
  cell{15}{1} = {r=2}{},
  cell{15}{2} = {c},
  cell{17}{1} = {r=2}{},
  cell{17}{2} = {c},
  hline{1,19} = {-}{0.08em},
  hline{2} = {-}{0.05em},
  hline{9,15,17} = {-}{dotted},
}
\textbf{Parameter}   & \textbf{Value}  \\
TF-IDF Max Features  & 100             \\
                     & 500             \\
                     & 1,000           \\
                     & 5,000           \\
                     & 10,000          \\
                     & \textbf{50,000} \\
                     & 100,00          \\
TF-IDF N-Grams Range & (1,1)           \\
                     & (1,2)           \\
                     & (1,3)           \\
                     & (1,4)           \\
                     & \textbf{(1,5)}  \\
                     & (1,10)          \\
TF-IDF Lower Case    & True            \\
                     & \textbf{False}  \\
TF-IDF Analyzer      & \textbf{Word}   \\
                     & Char            
\end{tblr}
\caption{List of hyperparameters tested besides delexicalization. The usage of bold highlights the best result obtained. The parameters name follows the \texttt{sklearn} convention}
\label{tab:hyperparameters}
\end{table}

\section{Annotation Results}
\label{app:annotation}

In Table~\ref{tab:annotations_detailed} we detail the annotation agreement metrics per-domain for the manually label subset of the PtBrVId corpus. The table shows statistics for the Fleiss' Kappa with all the labels and the Fleiss' Kappa when the entries for which one of the annotators marked the entry as ``Undetermined''. To complete the table we also show the percentega of entries for which at least one annotator labeled as ``Undetermined''.  

Table~\ref{tab:annotations_detailed} provides a detailed breakdown of the annotation agreement metrics per domain for the manually labeled subset of the PtBrVId corpus. The table presents statistics for Fleiss' Kappa across all labels and Fleiss' Kappa calculated after excluding entries where at least one annotator marked the entry as ``Undetermined.'' Additionally, the table includes the percentage of entries labeled as ``Undetermined'' by at least one annotator.

\input{tables/iaa_domain}

The low results in the literature domain are explained by its compilation of non-contemporary books. In the 18th and 19th century, the cultural differences between Portuguese and Brazilian writers were less significant, and therefore it creates additional uncertainty. One avenue to further improve the quality of  the models would be to integrate contemporary literature to the dataset.

\section{Computational Resources}

This study relied on Google Cloud N1 Compute Engines to perform the tuning and training of both the baseline and the BERT architecture. For the baseline, no GPU was needed, and it was used N1 instances with 192 CPU cores and 1024 GB of RAM. While for BERT we used an instance with 16 CPU cores, 30 GB of RAM and 4x Tesla T4. The grid search on N-grams takes approximately three hours in such conditions, and for BERT it takes approximately 52 hours to finish. The final training took three hours for N-grams and approximately ten hours for BERT.
